# Supplementary material for: Optimal and Robust Waveform Design for MIMO-OFDM Channel Sensing: A Cram\'er-Rao Bound Perspective
Source: arXiv:2301.10689 source file (2023-01-25)
Supplement: Supplementary file 1 [file appendix_lemma1.tex]

Suppose there is a set of waveforms $\hat{\bm{x}}_1, \hat{\bm{x}}_2, \dots, \hat{\bm{x}}_M$ with $\sum_m\|\hat{\bm{x}}_m\|^2_2< MP$. As $MP\le \sum_mP_m$, there should be a subset of waveforms $\brcur{\hat{\bm{x}}_{m_i}}_{i=1}^I$ with $\|\hat{\bm{x}}_{m_i}\|_2^2< P_{m_i}$. Thus, we can always find a new set of waveforms $\hat{\hat{\bm{x}}}_m = \beta_m\hat{\bm{x}}_m$ with $\beta_{m_j} > 1$ for $j\in J \subset \brcur{1\dots I}$ and $\beta_m = 1$ for else such that $\sum_m\|\hat{\hat{\bm{x}}}_m\|^2= MP$. It's then easy to verify that
\begin{equation}
    \sum_{m=1}^M \frac{2}{\sigma_m^2} \bm{\Lambda}_m\herm \bm{T}\herm \hat{\hat{\bm{x}}}_m^*\hat{\hat{\bm{x}}}_m^\top \bm{T\Lambda}_m \succ \sum_{m=1}^M \frac{2}{\sigma_m^2}\bm{\Lambda}_m\herm \bm{T}\herm \hat{\bm{x}}_m^*\hat{\bm{x}}_m^\top \bm{T\Lambda}_m
\end{equation}
and we use the property that the Hadamard product of two PSD matrices is still PSD to obtain
\begin{equation}
    \begin{split}
    &\re{\br{\frac{2}{\sigma_m^2}\sum_{m=1}^M \bm{\Lambda}_m\herm \bm{T}\herm \hat{\hat{\bm{x}}}_m^*\hat{\hat{\bm{x}}}_m^\top \bm{T\Lambda}_m}\circ \br{\bm{R}\herm \bm{R}}} \succ\\
    &\quad\re{\br{\frac{2}{\sigma_m^2}\sum_{m=1}^M \bm{\Lambda}_m\herm \bm{T}\herm \hat{\bm{x}}_m^*\hat{\bm{x}}_m^\top \bm{T\Lambda}_m}\circ \br{\bm{R}\herm \bm{R}}}
    \end{split}
\end{equation}
due to the linearity of Hadamard product and the $\re{\cdot}$ operation. Since $\det\brcur{\bm{A}} > \det \{\bm{B}\}$ if $\bm{A} \succ \bm{B}$ we conclude the validity for problem \eqref{P1}.
